# Supplementary material for: Identification of Patient Zero in Static and Temporal Networks - Robustness and Limitations
Source: arXiv:1406.2909 ancillary file (2015-06-11)
Supplement: Supplementary file 1 [file SupplementalMaterial.pdf]

# Supplemental Material: Identification of Patient Zero in Static and Temporal Networks - Robustness and Limitations

Nino Antulov-Fantulin[1], Alen Lančić[2], Tomislav Šmuc[1], Hrvoje Štefančić[3,4], and Mile Šikić[5,6]

[1]Computational Biology and Bioinformatics Group, Division of Electronics, Rudjer Bošković Institute, Zagreb, Croatia
[2]Faculty of Science, Department of Mathematics, University of Zagreb, Croatia
[3]Theoretical Physics Division, Rudjer Bošković Institute, Zagreb, Croatia
[4]Catholic University of Croatia, Zagreb, Croatia
[5]Faculty of Electrical Engineering and Computing, Department of Electronic Systems and Information Processing, University of Zagreb, Croatia
[6]Bioinformatics Institute, A*STAR, Singapore, Republic of Singapore

June 11, 2015

## Contents

**1 Analytical combinatorics approach** **2**

**2 Direct Monte Carlo estimator and pruning** **9**

**3 Benchmark analysis** **11**

**4 Benchmark dataset** **15**

**5 Soft Margin implementation details** **16**

**6 Pruning and Soft Margin** **18**

**7 Soft Margin time complexity** **19**

**8 Empirical temporal network – description** **20**

**9 Source detection on temporal networks** **20**

**10 Detectability regimes** **22**

# 1 Analytical combinatorics approach

In this section, we describe the general procedure for calculating exact source probability distributions by using the formalism of generating functions. We start, by introducing all needed definitions and suitable notations for this approach. Let $G = (V, E)$ be a given graph and $v_i, v_j \in V, i \neq j$. We define the discrete sample space $\Omega$ of elementary events for stochastic epidemic spreading on $G$ as the Cartesian product of elementary events on each edge $(v_i, v_j)$: (i) disease propagated from node $v_i$ to node $v_j$, (ii) disease propagated from node $v_j$ to node $v_i$ and (iii) disease did not propagate through the edge.

Let $SP_{(i,j)} = \left\{w_{(i,j),k} : 1 \leqslant k \leqslant m_{i,j}\right\}$ be the set of all simple paths $w_{(i,j),k}$ (with cardinality $m_{i,j}$) in $G$ beginning at $v_i$ and ending at $v_j$. Let $W_{(i,j),k}$ denote the event in which the epidemic process has passed through each edge consequently for all vertices in $w_{(i,j),k}$ in the appropriate direction, while we don't put any restrictions on the spreading of the epidemic for other edges in the graph. We will use the SIR model as the main contagion model, which is parametrized by the probability $p$ that an infected node infects a susceptible neighbour node and by the probability $q$ that an infected node recovers in one discrete time step.

Now, let's define the event $i \to j$ as $\bigcup\limits_{k=1}^{m_{i,j}} W_{(i,j),k}$; intuitively, that is an event in which the vertex $v_i$ has become infected during the epidemic process (possibly as the initial source of the epidemic), after which the epidemic has spread to the vertex $v_j$.

We define a realization $r$ as a function $r : V \to \{0, 1\}$ such that $r(v_k) = 1$ if $v_k$ was infected during the epidemic process and $r(v_k) = 0$ otherwise. Now, let's define the random vector $R$ which describes the state of all vertices at the end of the epidemic, and the random variable $I$ which describes a choice of the initial source of the epidemic. Note, that in the main manuscript we have used the following notation: $\vec{r}$ for realization, $\vec{R}$ for random vector and $\Theta$ for the source nodes, but only in this section due to the simplicity of notation in analytical formulas we use the equivalent notation $r$, $R$ and $I$. We have

$$\mathbb{P}(R = r|I = i) = \mathbb{P}((\bigcap_{v_j \in r^{-1}(1)} i \to j) \cap (\bigcap_{v_k \in r^{-1}(0)} (i \to k)^C)\,|I = i) =$$

$$\mathbb{P}(\bigcap_{v_j \in r^{-1}(1)} (\bigcup_{\ell=1}^{m_{i,j}} W_{(i,j),\ell}) \cap (\bigcap_{v_k \in r^{-1}(0)} (i \to k)^C)\,|I = i) \overset{S_{r,i} := \left\{g \in \mathbb{N}^{\left(r^{-1}(1)\right)} : g(v_j) \in \{1,2,\ldots,m_{i,j}\}\right\}}{=},$$

where $S_{r,i}$ is a set of functions defined on $r^{-1}(1)$ (nodes infected in $r$) such that each function maps a vertex in $r^{-1}(1)$ to an index of a path from the source $i$ to that vertex. The cardinality $|S_{r,i}|$ of the set $S_{r,i}$ is equal to the product of the number of simple paths $m_{i,j}$ from node $i$ to all other nodes $j$ in the set $r^{-1}(1)$. In order to get a better intuition about the set $S_{r,i}$ see the Example 2 from this section.

$$\mathbb{P}(\bigcup_{\psi \in S_{r,i}} (\bigcap_{v_\kappa \in r^{-1}(1)} W_{(i,\kappa),\psi(v_\kappa)}) \cap (\bigcap_{v_k \in r^{-1}(0)} (i \to k)^C)\,|I = i) \overset{\text{inclusion - exclusion}}{\underset{\text{principle}}{=}}$$

$$\sum_{\ell=1}^{|S_{r,i}|} \sum_{J \subseteq S_{r,i}, |J| = \ell} (-1)^{\ell-1} \mathbb{P}((\bigcap_{\psi \in J} \bigcap_{v_\kappa \in r^{-1}(1)} W_{(i,\kappa),\psi(v_\kappa)}) \cap (\bigcap_{v_k \in r^{-1}(0)} (i \to k)^C)\,|I = i)$$

For practical purposes, it is useful to note that $(\bigcap_{\psi \in J} \bigcap_{v_\kappa \in r^{-1}(1)} W_{(i,\kappa),\psi(v_\kappa)}) \cap \bigcap_{v_k \in r^{-1}(0)} (i \to k)^C = \bigcap_{\psi \in J} (\bigcap_{v_\kappa \in r^{-1}(1)} (W_{(i,k),\psi(v_\kappa)} \cap \bigcap_{v_k \in r^{-1}(0)} (i \to k)^C))$. In conclusion, to be able to evaluate $\mathbb{P}(R = r|I = i)$, it suffices to be able to evaluate terms of the form $\mathbb{P}(\bigcap_{\psi \in J} (\bigcap_{v_\kappa \in r^{-1}(1)} (W_{(i,\kappa),\psi(v_\kappa)} \cap \bigcap_{v_k \in r^{-1}(0)} (i \to k)^C))\,|I = i)$. We will now proceed to describe how to obtain their values using generating functions.

For a given vertex $v$, where $n-k$ is the number of edges incident to $v$ through which infection may be spread (edges which eventually transmit the infection to $v$ are not eligible) but is not spread, we observe the probability of the event that, for the first time after the moment of its infection, through predetermined $k$ (ordered) edges the infection spreads successively after $i_1, i_2, \ldots, i_k$ time steps (in the same order), while it does not spread through the remaining $n-k$ edges, in case that until the end of the simulation from the step of initial infection of the vertex $v$ there remains $l$ steps. Note that any number of edges on which no restrictions are placed are also allowed, since they do not affect the calculation in any way. We denote that event as $(Y_1, Y_2, \ldots, Y_k, t_R) = (i_1, \ldots, i_k, l)$. The corresponding generating function of a multivariate sequence of the form $\mathbb{P}\left((Y_1, Y_2, \ldots, Y_k, t_R) = (i_1, \ldots, i_k, l)\right)$ is

$$f_{X_n=k}\left(x_1, \ldots, x_k, r\right) =$$

$$\sum_{i_1,\ldots,i_k,l} \mathbb{P}\left((Y_1, Y_2, \ldots, Y_k, t_R) = (i_1, \ldots, i_k, l)\right) r^l \prod_{j=1}^{k} x_j^{i_j} = \sum_{l=0}^{\infty} \left( \sum_{i_1,\ldots,i_k} \mathbb{P}\left((Y_1, Y_2, \ldots, Y_k) = (i_1, \ldots, i_k) \,|t_R = l\right) \prod_{j=1}^{k} x_j^{i_j} \right) \mathbb{P}\left(t_R = l\right) r^l$$

If $T_v$ is a number of steps from the initial infection of the vertex $v$ until its recovery, we have

$$\sum_{i_1,\ldots,i_k} \mathbb{P}\left((Y_1, \ldots, Y_k) = (i_1, \ldots, i_k) \,|t_R = l\right) \prod_{j=1}^{k} x_j^{i_j} =$$

$$= \sum_{i_1,\ldots,i_k} \left( \sum_{m=1}^{l} \mathbb{P}\left((Y_1, \ldots, Y_k) = (i_1, \ldots, i_k), T_v = m | t_R = l\right) + \mathbb{P}\left((Y_1, \ldots, Y_k) = (i_1, \ldots, i_k), T_v > l | t_R = l\right) \right) \prod_{j=1}^{k} x_j^{i_j}$$

and since $Y_1, \ldots, Y_k$ are mutually conditionally independent given $T_v$, we have

$$\sum_{i_1,\ldots,i_k} \mathbb{P}\left((Y_1, Y_2, \ldots, Y_k) = (i_1, \ldots, i_k) \,|t_R = l\right) \prod_{j=1}^{k} x_j^{i_j} = \sum_{m=1}^{l} \sum_{1 \leqslant i_1,\ldots,i_k \leqslant m} \mathbb{P}\left(T_v = m\right) (1-p)^{(n-k)m} \prod_{j=1}^{k} \mathbb{P}\left(Y_j = i_j | T_v = m, t_{R=l}\right) x_j^{i_j} +$$

$$+ \mathbb{P}\left(T_v > l\right) (1-p)^{(n-k)l} \sum_{1 \leqslant i_1,\ldots,i_k \leqslant l} \prod_{j=1}^{k} \mathbb{P}\left(Y_j = i_j | T_v > l, t_R = l\right) x_j^{i_j} =$$

$$= q\sum_{m=1}^{l}\sum_{1\leqslant i_1,\dots,i_k\leqslant m}(1-q)^{m-1}(1-p)^{(n-k)m}\prod_{j=1}^{k}p(1-p)^{i_j-1}x_j^{i_j}+(1-q)^l(1-p)^{(n-k)l}\sum_{1\leqslant i_1,\dots,i_k\leqslant l}\prod_{j=1}^{k}p(1-p)^{i_j-1}x_j^{i_j} =$$

$$q\sum_{m=1}^{l}(1-q)^{m-1}(1-p)^{(n-k)m}\prod_{j=1}^{k}p\sum_{i_j=1}^{m}(1-p)^{i_j-1}x_j^{i_j}+(1-q)^l(1-p)^{(n-k)l}\prod_{j=1}^{k}p\sum_{i_j=1}^{l}(1-p)^{i_j-1}x_j^{i_j}.$$

$$f_{X_n=k}(x_1,\dots,x_k,r) =$$
$$\sum_{l=0}^{\infty}\left(q\sum_{m=1}^{l}(1-q)^{m-1}(1-p)^{(n-k)m}\prod_{j=1}^{k}p\sum_{i_j=1}^{m}(1-p)^{i_j-1}x_j^{i_j}+(1-q)^l(1-p)^{(n-k)l}\prod_{j=1}^{k}p\sum_{i_j=1}^{l}(1-p)^{i_j-1}x_j^{i_j}\right)r^l\mathbb{P}(t_R=l)$$

The equality above motivates the following definition:

$$F_{X_n=k}(x_1,\dots,x_k,r) :=$$
$$\sum_{l=0}^{\infty}\left(q\sum_{m=1}^{l}(1-q)^{m-1}(1-p)^{(n-k)m}\prod_{j=1}^{k}p\sum_{i_j=1}^{m}(1-p)^{i_j-1}x_j^{i_j}+(1-q)^l(1-p)^{(n-k)l}\prod_{j=1}^{k}p\sum_{i_j=1}^{l}(1-p)^{i_j-1}x_j^{i_j}\right)r^l. \qquad (1)$$

Note that $F$ is the generating function corresponding to a multivariate sequence of the form $\mathbb{P}((Y_1,Y_2,\dots,Y_k)=(i_1,\dots,i_k)\,|t_R=l)$. The factor $\mathbb{P}(t_R=l)$ in $f$ follows from the information on the spreading process along the paths from the initially infected node to the observed node and it is calculated from the corresponding products of $F$ functions for nodes on these paths (see Example 1).

In further calculations, it's important to know the values of particular coefficients denoted as $\langle x_1^{i_1}\dots x_k^{i_k}r^l\rangle$ of the generating function defined as above. From (1) we obtain the following coefficients:

$$\left\langle x_1^{i_1}\ldots x_k^{i_k} r^l\right\rangle F_{X_n=k}\left(x_1,\ldots,x_k,r\right)=$$
$$k=0,l=0\Rightarrow\left\langle x_1^{i_1}\ldots x_k^{i_k} r^l\right\rangle F_{X_n=k}\left(x_1,\ldots,x_k,r\right)=1$$
$$k>0,l=0\Rightarrow\left\langle x_1^{i_1}\ldots x_k^{i_k} r^l\right\rangle F_{X_n=k}\left(x_1,\ldots,x_k,r\right)=0$$
$$k=0,l>0\Rightarrow\left\langle x_1^{i_1}\ldots x_k^{i_k} r^l\right\rangle F_{X_n=k}\left(x_1,\ldots,x_k,r\right)=(1-q)^l(1-p)^{nl}+q\frac{(1-p)^n-(1-q)^l(1-p)^{(l+1)n}}{1-(1-q)\,(1-p)^n}$$
$$k>0,l>0\Rightarrow\left\langle x_1^{i_1}\ldots x_k^{i_k} r^l\right\rangle F_{X_n=k}\left(x_1,\ldots,x_k,r\right)=$$
$$p^k(1-q)^l(1-p)^{l(n-k)}(1-p)^{i_1+\ldots+i_k-k}+qp^k(1-p)^{i_1+\ldots+i_k-k}\sum_{m=\max\{i_1,\ldots,i_k\}}^{l}(1-q)^{m-1}(1-p)^{m(n-k)}=$$
$$p^k(1-p)^{i_1+\ldots+i_k-k}[(1-q)^l(1-p)^{l(n-k)}+q\sum_{m=\max\{i_1,\ldots,i_k\}}^{l}(1-q)^{m-1}(1-p)^{m(n-k)}]=$$
$$p^k(1-p)^{i_1+\ldots+i_k-k}[(1-q)^l(1-p)^{l(n-k)}+q\frac{(1-q)^{\max\{i_1,\ldots,i_k\}-1}(1-p)^{(n-k)\max\{i_1,\ldots,i_k\}}-(1-q)^l(1-p)^{(l+1)(n-k)}}{1-(1-q)\,(1-p)^{n-k}}]$$

When we calculate $\mathbb{P}(\bigcap_{\psi\in J}(\bigcap_{v_\kappa\in r^{-1}(1)}(W_{(i,\kappa),\psi(v_\kappa)}\cap\bigcap_{v_k\in r^{-1}(0)}(i\to k)^C))\,|I=i)$, each vertex $v\in r^{-1}(1)\setminus\{v_i\}$ has at least one adjacent vertex which transmits the infection to it; let $v_1,\ldots,v_\eta$ be all such vertices, $l_1,\ldots,l_\eta$ be the times left from the time of their initial infection until the end of the simulation and $j_1,\ldots,j_\eta$ be the times when they first transmitted the infection to $v$ counting from time of their initial infection. Then, we easily get the time $l$ remaining from the moment of initial infection of the vertex $v$ until the end of the simulation as $\min_{1\leqslant k\leqslant\eta}(l_k-j_k)$. Since the product of generating functions corresponds to convolution of their sequences, it's easy to see that, in its coefficients, a product of generating functions defined as above contains all information we need to calculate $\mathbb{P}(\bigcap_{\psi\in J}(\bigcap_{v_\kappa\in r^{-1}(1)}(W_{(i,\kappa),\psi(v_\kappa)}\cap\bigcap_{v_k\in r^{-1}(0)}(i\to k)^C))\,|I=i)$.

**Example 1:**

For a specific realization from Supplementary Figure 1, we can calculate the probability of each vertex being the source of the epidemic. We assign to each node $i$ "dummy" variables $r_i$, and to each edge a "dummy" variable $x_k$, the restriction being that the first time of vertex' infection plus the time remaining to the end of the simulation always equals $T$ and that first time of infection transmission through any edge (counting from the first time of infection of the spreading vertex) can not be greater than the time remaining until the end of the simulation (also counting from the first time of infection of the spreading vertex). For $t = 5, p = 0.2, q = 0.3$ we get:

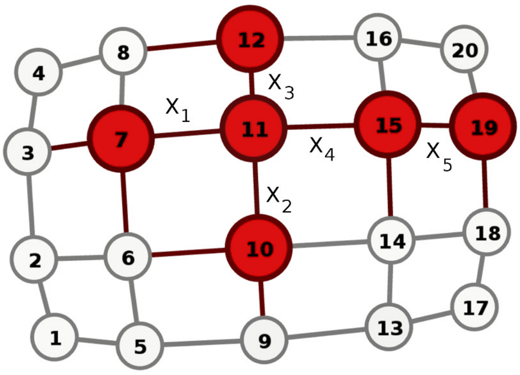


Supplementary Figure 1: Realization on grid network, where the infected nodes are coloured with red.

$$P\left(R=r|I=7,T=t\right)=$$

$$\sum_{n_1=1}^{t}\sum_{n_2=1}^{t-n_1}\sum_{n_3=1}^{t-n_1}\sum_{n_4=1}^{t-n_1}\sum_{n_5=1}^{t-n_1-n_4}\left\langle r_7^t x_1^{n_1} r_{11}^{t-n_1} x_2^{n_2} r_{10}^{t-n_1-n_2} x_3^{n_3} r_{12}^{t-n_1-n_3} x_4^{n_4} r_{15}^{t-n_1-n_4} x_5^{n_5} r_{19}^{t-n_1-n_4-n_5}\right\rangle$$

$$F_{X_4=1}\left(x_1,r_7\right)F_{X_3=3}\left(x_2,x_3,x_4,r_{11}\right)F_{X_3=0}\left(r_{10}\right)F_{X_2=0}\left(r_{12}\right)F_{X_3=1}\left(x_5,r_{15}\right)F_{X_2=0}\left(r_{19}\right)=0.0001368350$$

$$P\left(R=r|I=11,T=t\right)=$$

$$\sum_{n_1=1}^{t}\sum_{n_2=1}^{t}\sum_{n_3=1}^{t}\sum_{n_4=1}^{t}\sum_{n_5=1}^{t-n_4}\left\langle r_{11}^t x_1^{n_1} r_7^{t-n_1} x_2^{n_2} r_{10}^{t-n_2} x_3^{n_3} r_{12}^{t-n_3} x_4^{n_4} r_{15}^{t-n_4} x_5^{n_5} r_{19}^{t-n_4-n_5}\right\rangle$$

$$F_{X_4=4}\left(x_1,x_2,x_3,x_4,r_{11}\right)F_{X_3=0}\left(r_7\right)F_{X_2=0}\left(r_{12}\right)F_{X_3=0}\left(r_{10}\right)F_{X_3=1}\left(x_5,r_{15}\right)F_{X_2=0}\left(r_{19}\right)=0.0003924644$$

$$P\left(R=r|I=10,T=t\right)=$$

$$\sum_{n_2=1}^{t}\sum_{n_1=1}^{t-n_2}\sum_{n_3=1}^{t-n_2}\sum_{n_4=1}^{t-n_2}\sum_{n_5=1}^{t-n_2-n_4}\left\langle r_{10}^t x_2^{n_2} r_{11}^{t-n_2} x_1^{n_1} r_7^{t-n_2-n_1} x_3^{n_3} r_{12}^{t-n_2-n_3} x_4^{n_4} r_{15}^{t-n_2-n_4} x_5^{n_5} r_{19}^{t-n_2-n_4-n_5}\right\rangle$$

$$F_{X_4=1}\left(x_2,r_{10}\right)F_{X_3=3}\left(x_1,x_3,x_4,r_{11}\right)F_{X_3=0}\left(r_7\right)F_{X_2=0}\left(r_{12}\right)F_{X_3=1}\left(x_5,r_{15}\right)F_{X_2=0}\left(r_{19}\right)=0.0001368350$$

$$P\left(R=r|I=12,T=t\right)=$$

$$\sum_{n_3=1}^{t}\sum_{n_1=1}^{t-n_3}\sum_{n_2=1}^{t-n_3}\sum_{n_4=1}^{t-n_3}\sum_{n_5=1}^{t-n_3-n_4}\left\langle r_{12}^t x_3^{n_3} r_{11}^{t-n_3} x_1^{n_1} r_7^{t-n_3-n_1} x_2^{n_2} r_{10}^{t-n_3-n_2} x_4^{n_4} r_{15}^{t-n_3-n_4} x_5^{n_5} r_{19}^{t-n_3-n_4-n_5}\right\rangle$$

$$F_{X_3=1}\left(x_3,r_{12}\right)F_{X_3=3}\left(x_1,x_2,x_4,r_{11}\right)F_{X_3=0}\left(r_7\right)F_{X_3=0}\left(r_{10}\right)F_{X_3=1}\left(x_5,r_{15}\right)F_{X_2=0}\left(r_{19}\right)=0.0001772788$$

$$P\left(R=r|I=15,T=t\right)=$$

$$\sum_{n_5=1}^{t}\sum_{n_4=1}^{t}\sum_{n_1=1}^{t-n_4}\sum_{n_2=1}^{t-n_4}\sum_{n_3=1}^{t-n_4}\left\langle r_{15}^{t}x_5^{n_5}r_{19}^{t-n_5}x_4^{n_4}r_{11}^{t-n_4}x_1^{n_1}r_7^{t-n_4-n_1}x_2^{n_2}r_{10}^{t-n_4-n_2}x_3^{n_3}r_{12}^{t-n_4-n_3}\right\rangle$$

$$F_{X_4=2}\left(x_4,x_5,r_{15}\right)F_{X_2=0}\left(r_{19}\right)F_{X_3=3}\left(x_1,x_2,x_3,r_{11}\right)F_{X_3=0}\left(r_7\right)F_{X_3=0}\left(r_{10}\right)F_{X_2=0}\left(r_{12}\right)=0.0002219489$$

$$P\left(R=r|I=19,T=t\right)=$$

$$\sum_{n_5=1}^{t}\sum_{n_4=1}^{t-n_5}\sum_{n_1=1}^{t-n_4-n_5}\sum_{n_2=1}^{t-n_4-n_5}\sum_{n_3=1}^{t-n_4-n_5}\left\langle r_{19}^{t}x_5^{n_5}r_{15}^{t-n_5}x_4^{n_4}r_{11}^{t-n_5-n_4}x_1^{n_1}r_7^{t-n_5-n_4-n_1}x_2^{n_2}r_{10}^{t-n_5-n_4-n_2}x_3^{n_3}r_{12}^{t-n_5-n_4-n_3}\right\rangle$$

$$F_{X_3=1}\left(x_5,r_{19}\right)F_{X_3=1}\left(x_4,r_{15}\right)F_{X_3=3}\left(x_1,x_2,x_3,r_{11}\right)F_{X_3=0}\left(r_{10}\right)F_{X_3=0}\left(r_7\right)F_{X_2=0}\left(r_{12}\right)=0.0001553419$$

The script in Wolfram Mathematica that calculates source likelihoods for this toy example is downloadable here[1]. The probability distribution over sources we get via Bayes formula:

$$P(I=i|\vec{R}=\vec{r}_*)=\frac{P(\vec{R}=\vec{r}_*|I=i)P(I=i)}{\sum_j P(\vec{R}=\vec{r}_*|I=j)P(I=j)},$$

and since our prior source probabilities are equal we get:

$$P(I=i|\vec{R}=\vec{r}_*)=\frac{P(\vec{R}=\vec{r}_*|I=i)}{\sum_j P(\vec{R}=\vec{r}_*|I=j)}.$$

In Figure 2, Plot A, we demonstrate the non-uniqueness of single source solution for the realization in Plot B and the correspondence (maximal absolute difference $< 10^{-10}$) between the direct Monte-Carlo and analytical combinatorics.

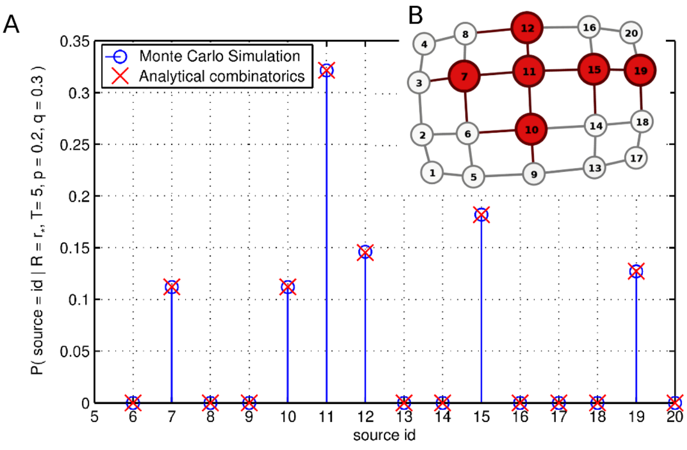


Supplementary Figure 2: Plot A: The realization $\vec{r_*}$ of SIR contagion process ($p=0.2, q=0.3, T=5$) on a small 4-connected lattice. The infected nodes in the realization are denoted with red colour and each node is denoted with its identification number. Plot B: The source probability distribution $P(\Theta=\theta_i|\vec{R}=\vec{r}_*)$ for a given realization $\vec{r_*}$. The solution is calculated with the direct Monte-Carlo estimator with $n=10^9$ simulations per node and verified by the analytical combinatoric method (generating functions).

**Example 2:**
Now, let us consider a simple network with the source node $v_1$ and the following infected nodes $r^{-1}(1)=\{v_1,v_2,v_3,v_4\}$.

[1] http://lis.irb.hr/epidemic/

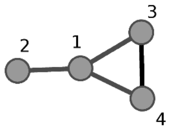


| $x$ | $v_2$ | $v_3$ | $v_4$ |
|---|---|---|---|
| $\psi_1(x)$ | 1 | 1 | 1 |
| $\psi_2(x)$ | 1 | 2 | 1 |
| $\psi_3(x)$ | 1 | 1 | 2 |
| $\psi_4(x)$ | 1 | 2 | 2 |

Now we enumerate simple paths from the source node $v_1$ to all other infected nodes. From node $v_1$ there exist only one simple path $W_{(1,2),1}$ to node $v_2$. From node $v_1$ there exist only two simple paths: $W_{(1,3),1}$ and $W_{(1,3),2}$ to node $v_3$. From node $v_1$ there exists only two simple paths: $W_{(1,4),1}$ and $W_{(1,4),2}$ to node $v_4$. The set $S_{r,1} = \{\psi_1(x), \psi_2(x), \psi_3(x), \psi_4(x)\}$ consists out of all the functions defined on $r^{-1}(1)$ (nodes infected in $r$) such that each function maps a vertex in $r^{-1}(1)$ to an index of a path from the source 1 to that vertex, as denoted in the table above.
Let us recall the formula which is used to calculate the source probability:

$$\mathbb{P}(R = r|I = i) = \mathbb{P}((\bigcap_{v_j \in r^{-1}(1)} i \to j) \cap (\bigcap_{v_k \in r^{-1}(0)} (i \to k)^C)\,|I = i).$$

We will now just expand the first term in this formula for our specific example for node $i = 1$.

$$\bigcap_{v_j \in r^{-1}(1)} i \to j = \bigcap_{v_j \in r^{-1}(1)} (\bigcup_{\ell=1}^{m_{i,j}} W_{(i,j),\ell}) = (W_{(1,2),1}) \cap (W_{(1,3),1} \cup W_{(1,3),2}) \cap (W_{(1,4),1} \cup W_{(1,4),2})$$

$$= \underbrace{(\overbrace{(W_{(1,2),1} \cap W_{(1,3),1})}^{B} \cup \overbrace{(W_{(1,2),1} \cup W_{(1,3),2})}^{C})}_{A} \cap (W_{(1,4),1} \cup W_{(1,4),2}) = (A \cap W_{(1,4),1}) \cup (A \cap W_{(1,4),2})$$

$$= ((B \cup C) \cap W_{(1,4),1}) \cup ((B \cup C) \cap W_{(1,4),2}) = (B \cap W_{(1,4),1}) \cup (C \cap W_{(1,4),1}) \cup (B \cap W_{(1,4),2}) \cup (C \cap W_{(1,4),2})$$

$$= (W_{(1,2),1} \cap W_{(1,3),1} \cap W_{(1,4),1}) \cup (W_{(1,2),1} \cap W_{(1,3),2} \cap W_{(1,4),1}) \cup (W_{(1,2),1} \cap W_{(1,3),1} \cap W_{(1,4),2}) \cup$$

$$\cup (W_{(1,2),1} \cap W_{(1,3),2} \cap W_{(1,4),2}) = \bigcup_{\psi \in S_{r,1}} (\bigcap_{v_\kappa \in r^{-1}(1)} W_{(i,\kappa),\psi(v_\kappa)})$$

Now, we will explicitly write down a few events on this graph. The event is the Cartesian product of elementary events on each edge $(v_i, v_j)$: (i) "$\to$" disease propagated from node $v_i$ to node $v_j$, (ii) "$\leftarrow$"disease propagated from node $v_j$ to node $v_i$ and (iii) "$||$"disease did not propagate through the edge. The events are written down as a Cartesian product on edges: $(v_1, v_2), (v_1, v_3), (v_1, v_4), (v_3, v_4)$. For example the event:

$$W_{(3,2),1} = \{\to\} \times \{\leftarrow\} \times \{\to, \leftarrow, ||\} \times \{\to, \leftarrow, ||\},$$

describes the event of disease passing from node $v_1$ to $v_2$ and from $v_3$ to $v_1$ and no restrictions on other edges. We will now write few more events on this example:

$$W_{(1,2),1} = \{\to\} \times \{\to, \leftarrow, ||\} \times \{\to, \leftarrow, ||\} \times \{\to, \leftarrow, ||\},$$

$$W_{(1,2),1} \cap W_{(3,2),1} = \{\to\} \times \{\leftarrow\} \times \{\to, \leftarrow, ||\} \times \{\to, \leftarrow, ||\},$$

$$W^C_{(3,2),1} = X \cup Y \cup Z$$

$$X = \{\leftarrow, ||\} \times \{\to, ||\} \times \{\to, \leftarrow, ||\} \times \{\to, \leftarrow, ||\}$$

$$Y = \{\to\} \times \{\to, ||\} \times \{\to, \leftarrow, ||\} \times \{\to, \leftarrow, ||\}$$

$$Z = \{\leftarrow, ||\} \times \{\leftarrow\} \times \{\to, \leftarrow, ||\} \times \{\to, \leftarrow, ||\}.$$

## 2 Direct Monte Carlo estimator and pruning

With **the direct Monte Carlo simulation approach**, for each node $i$ from the realization $\vec{r}_*$ a large number $n$ of epidemic spreading simulations with duration $T$ is performed with $i$ as an epidemic source. The number of simulations $n_i$ which coincide with the realization $\vec{r}_*$ is recorded. After the simulations for all potential source nodes in the realization $\vec{r}_*$ are finished, the probability of the node $i$ being the source of the epidemic is calculated as $n_i / \sum_j n_j$. Here we devise the rule for pruning realizations at some temporal point $t < T$ whose contribution is zero. Let us also define the error term for every simulated realization $\vec{r_i^t}$ at some point in time $t < T$ w.r.t observed realization $\vec{r_*^T}$ at time $T$:

$$error_t(\vec{r_i^t}, \vec{r_*^T}) = \frac{1}{N} \sum_{k \in V} ((\vec{r_*^T}(k) == 0) \wedge (\vec{r_i^t}(k) == 1)). \tag{2}$$

The error term calculates the number of corresponding nodes which are non-infected in the observed realization $\vec{r_*^T}$ at time $T$ and infected in the simulated realization $\vec{r_i^t}$ at time $t$.

**Proposition**: Monte Carlo SIR realization simulation $\vec{r_i^t}$ at time $t < T$ can be terminated if the $error_t(\vec{r_i^t}, \vec{r_*^T}) > 0$ and it will have no effect on the final estimation.

Proof: If at time $t$ the error term $error_t(\vec{r_i^t}, \vec{r_*^T}) > 0$, then at time $T$ the error can only increase: $error_T(\vec{r_i^T}, \vec{r_*^T}) \geq error_t(\vec{r_i^t}, \vec{r_*^T})$ because the error term $error_t(\vec{r_i^t}, \vec{r_*^T})$ is monotonic increasing function w.r.t. time $t+1, t+2, ..., T$ and direct Monte Carlo estimator rejects any realization with positive error term: $error_T(\vec{r_i^T}, \vec{r_*^T}) > 0$ . The infected state $(\vec{r_i^t}(k) == 1)$ is absorbing state w.r.t time $t$. Once the node leaves the susceptible state it can not come back to it in the SIR model.

The pruning mechanism provides a substantial acceleration (see Supplementary Figure 3) without inducing any errors to our estimation.

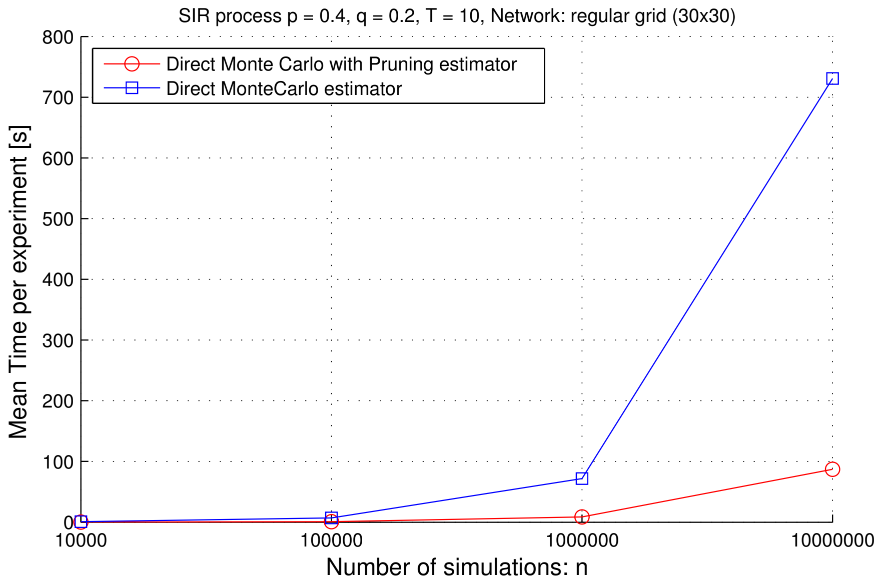


Supplementary Figure 3: The speed up of direct Monte Carlo estimation with the pruning rule for experiment with $n$ simulations per source node. Comparison of run-time per source detection experiment on 30 cpu cores(4 x AMD Opteron Processor 6134, 2.3 GHz with 8 cores each) averaged over 10 experiments.

The statistical significance of direct Monte-Carlo simulation results are controlled with the convergence conditions. We estimate two source PDFs, one ($P_i^n$) by doing $n$, and the other ($P_i^{2n}$) with $2n$ independent simulations, where $n$ is usually in the range $10^6 - 10^9$. Then, we choose the ML node as the node with the highest probability in ($P_i^{2n}$). The PDFs which satisfy the two following conditions:

$$|P_{ML}^{2n} - P_{ML}^{n}|/P_{ML}^{2n} \leq c, |P_i^n - P_i^{2n}| \leq c, \tag{3}$$

are said to converge with the direct Monte Carlo method. The relative error convergence with the value $c$ on all the nodes is a too strict computational condition for practical purposes as we are interested in finding the high probability source nodes.

## 3 Benchmark analysis

In order to do a proper comparison of different source detection estimators, there has to exist a proper measure of quality of solution. Because of the non-uniqueness of a single source node we will not compare the estimators by their ability to detect the true source, but instead by comparing their estimated source probabilities to the source probability distribution of the ideal algorithm. We have generated a series of benchmark cases for which we have calculated the probability distributions over the potential source candidates using the direct Monte Carlo estimator. Note that the direct Monte Carlo estimator has been validated by comparison with the analytical solution. In order to be sure that the direct Monte Carlo estimator outputs valid results on realizations with cycles, we set its convergence condition to $c = 0.05$. The convergence condition for direct Monte Carlo solution at $2x$ number of simulations was set to be: ML node relative error is: $|P_{ML}^{2x} - P_{ML}^{x}|/P_{ML}^{2x} \leq c$ and the maximal absolute error for all other nodes is: $|P_i^x - P_i^{2x}| \leq c$.

We have used a small 4-connected lattice ($N = 30 \times 30$) and SIR processes with different parameters $(p, q, T)$ with the direct Monte Carlo estimator with $[10^6 - 10^8]$ simulations per source, depending on the convergence condition, to obtain the source PDFs for our benchmark.

Next, we compare the representatives of three different classes of source detection estimators: network centrality estimators, belief propagation estimators and Monte Carlo estimators. For the network centrality estimation, we use the Jordan estimator [6], which assigns a weight to each potential node candidate which is equal to the maximal topological distance from the node candidate to all other infected nodes in a realization. Although the Jordan estimator uses a very simple rule, it outperforms most of other network centrality measures. The representative of the belief propagation estimators is the Dynamic Message Passing Algorithm (DMP) [1], which uses a mean-field-like approximation (independence approximation) about the node states along with a recursive analytical formula for the tree-like networks to estimate the source likelihoods.

Finally, we use our Soft Margin estimator which falls into the general class of the Monte Carlo estimators. Note that, when comparing the Soft Margin estimator, we evaluate it with a few orders of simulations less than the number of simulations used to generate the benchmark standard solution. The maximum likelihood (ML) node for each realization is determined by the benchmark solution. Then, for each estimator, we measure the ML accuracy performance and ML probability estimate error. The ML accuracy measures the expected number of times in which the estimators rank the ML node on rank 1 and relative ML error measures the ability to reconstruct the associated probability for the ML node. In Supplementary Figure 4, we can see the mean relative errors and the accuracy of the ML node for different estimators. From this analysis, we observe that the most estimators are trying to produce a valid ranking (ML accuracy) without estimating the true probability (ML relative error). The Soft Margin estimator is trying to estimate both the valid ranking and a valid probability at the same time. The source probability distribution for the observed realization contains more information about the initial conditions than just the ranking of potential candidates, especially for cases where the detectability limits are more pronounced.

Here, we provide the comparison of different estimators for the SIR model w.r.t. ML probability errors (see Supplementary Figure 6) and ML accuracy (see Supplementary Figure 7) on the benchmark dataset. The correct solutions were calculated with the direct Monte Carlo estimator with $[10^6 - 10^8]$ simulations per source depending on convergence condition. The convergence condition for direct Monte Carlo solution at $2x$ number of simulations was set to be: ML node relative error is: $|P_{ML}^{2x} - P_{ML}^{x}|/P_{ML}^{2x} \leq 0.05$ and the maximal absolute error for all other nodes is: $|P_i^x - P_i^{2x}| \leq 0.05$. We have compared the centrality-like estimators: Distance [7] and Jordan [6] centrality, Belief propagation estimator: DMP [1], different Monte Carlo estimators: AUCDF, AvgTopK and NaiveBayes [5] and two baseline solutions: Rnd (source likelihood is random number from [0,1]) and Const (all sources are equal).
Most of the aforementioned estimators do not output explicit source probability distribution function, but rather a ranking list with appropriate weights $w_i$, from which we calculate source pdf by re-normalization

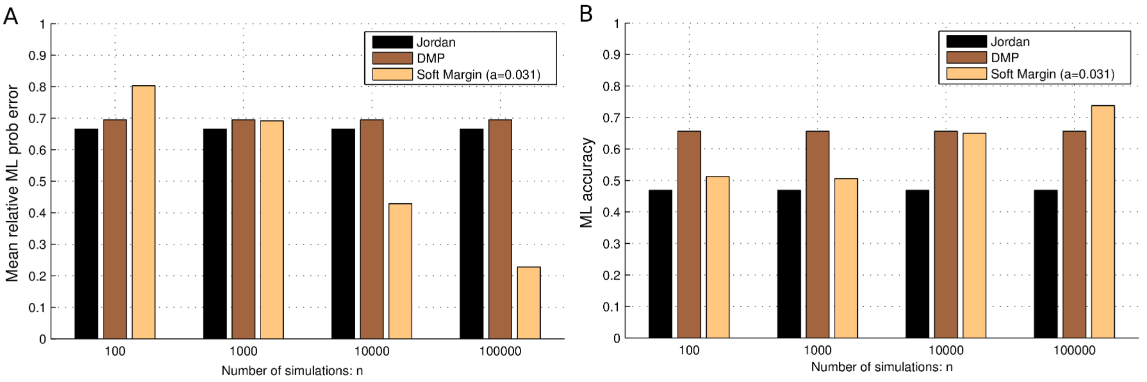


Supplementary Figure 4: Comparison of different estimators (Network centrality-Jordan, Belief Propagation-DMP and Monte Carlo-Soft Margin) performance with the ML relative probability estimation error (plot A) and ML accuracy (plot B) with the 160 different benchmark cases. Benchmark cases were calculated on a small 4-connected lattice with ($N = 30 \times 30$) and SIR process with different parameters $(p, q, T)$ with the direct Monte Carlo estimator with $[10^6 - 10^8]$ simulations per source depending on convergence condition with $c = 0.05$.

with factor $\sum_j w_j$ to get a PDF. We have used our implementation of distance [7], Jordan [6] centrality and Belief propagation estimator DMP [1].

In this manuscript, we use a conservative information about the node state at observed moment $t$, we only observe whether node is susceptible or not (realization $\vec{R}$ is a binary vector). This implies that we do not need additional information to distinguish whether node state is recovered or it is still infective. The original DMP [1] estimator additionally assumes that one can distinguish the recovered from infective state. Therefore, in order to apply the DMP [1] algorithm to our scenario, we had to adopt the estimation formula so that probability of node being infected is merged with probability of node being recovered in order to estimate the probability of being in either Infective or Recovered compartment. All other calculations were implemented according to the original algorithm [1]. In order to verify our implementation of the DMP algorithm, we have compared our DMP implementation on tree network, where the node state probability estimation should be correct. We have measured the difference between probability estimate that the node is susceptible after $T$ steps with the DMP and the SIR Monte Carlo simulation algorithm and we observe that less than 1 % of nodes have the relative error greater than 0.001, which means that the SIR Monte Carlo simulation algorithm estimates are very close to DMP on tree networks (see Supplementary Figure 5).

In a limit where the parameter $a \to 0$, for the Soft Margin estimator we obtain the unbiased estimate of the likelihood $P(\vec{R} = \vec{r}_*|\Theta = \theta)$. For cases when the parameter $a > 0$ we obtain an estimator which is estimating the likelihood by using the tail of pdf function $f(x)$ in a way that it uses the values of slightly different realizations to get estimate for observed realization $\vec{r_*}$. In Supplementary Figure 8 plot A and B, we can see the effect of different Soft Margin widths $a$ on the convergence. As the Soft Margin width parameter $a$ decreases, it becomes more similar to the unbiased estimator, but the convergence becomes slower.

In Figure 11, we show the phase diagram of entropy (1-detectability), for different value of $(p, q)$ and fixed stopping point $T$ on regular lattice. For each $(p, q)$ we plot the box plot and estimated probability density function of entropy over different realizations calculated with the Soft Margin estimator.

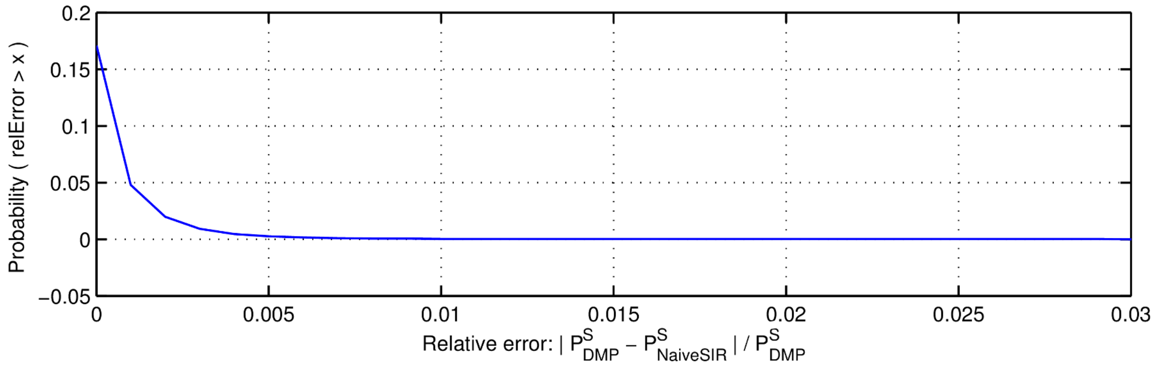


Supplementary Figure 5: Comparing Dynamic Message Passing (DMP) estimates of the node state probability for $p = 0.3, q = 0.5, T = 10$ with the SIR simulation estimates (NaiveSIR) on the Albert-Barabashi tree network ($N = 5000, m_0 = 2, m = 1$). Distribution of relative errors of node being susceptible with SIR simulation ($n = 10^4$) w.r.t. DMP on tree network.

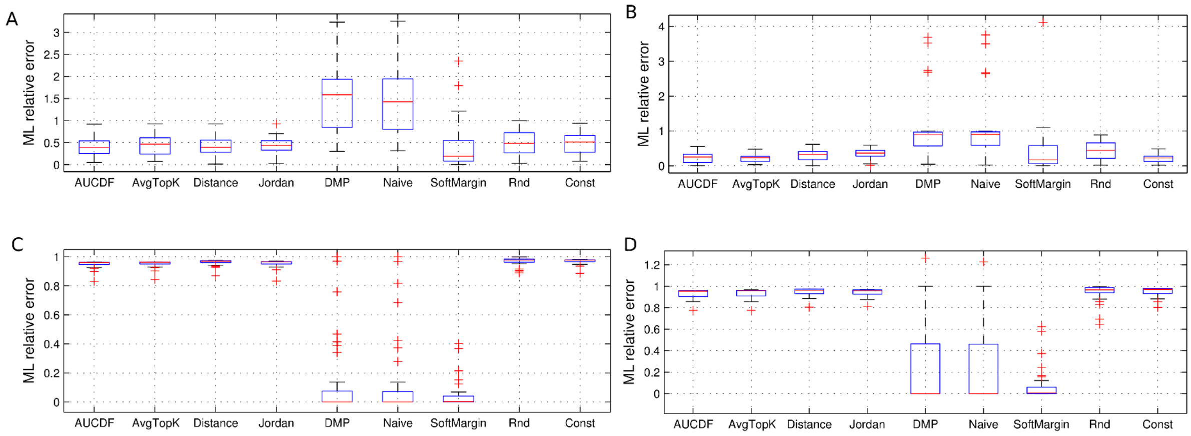


Supplementary Figure 6: The comparison of maximum likelihood probability errors with box-plots for different estimators and Soft Margin with $a = 0.031$. The error is relative error of maximum likelihood estimation w.r.t. gold standard ML probability obtained with direct Monte Carlo method for different parameters: $A = (p = 0.3, q = 0.3, T = 5)$, $B = (p = 0.3, q = 0.7, T = 5)$, $C = (p = 0.7, q = 0.3, T = 5)$ and $D = (p = 0.7, q = 0.7, T = 5)$.

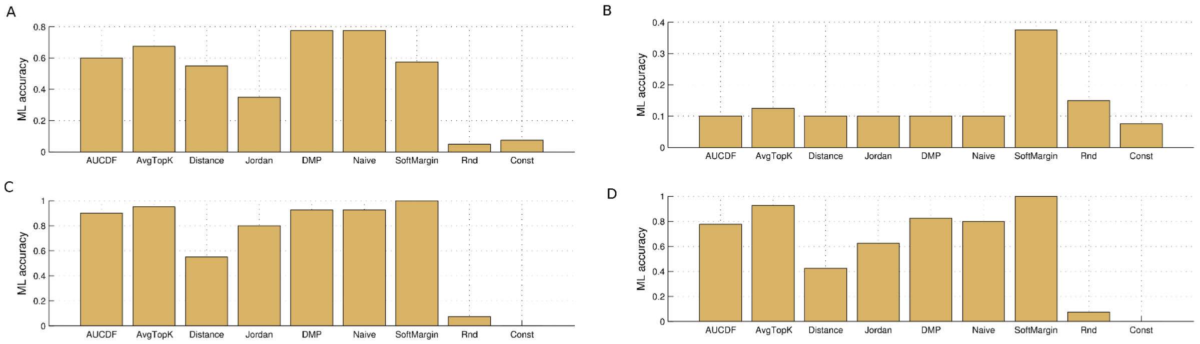


Supplementary Figure 7: The comparison of accuracy of detecting the maximum likelihood node with mean accuracy and standard deviation for different estimators and Soft Margin with $a = 0.031$. ML accuracy is the ratio of how many times the estimator ranks the ML node on rank 1 and total number of trials (ranking measure). plot A-D correspond to different parameters: $A = (p = 0.3, q = 0.3, T = 5)$, $B = (p = 0.3, q = 0.7, T = 5)$, $C = (p = 0.7, q = 0.3, T = 5)$ and $D = (p = 0.7, q = 0.7, T = 5)$.

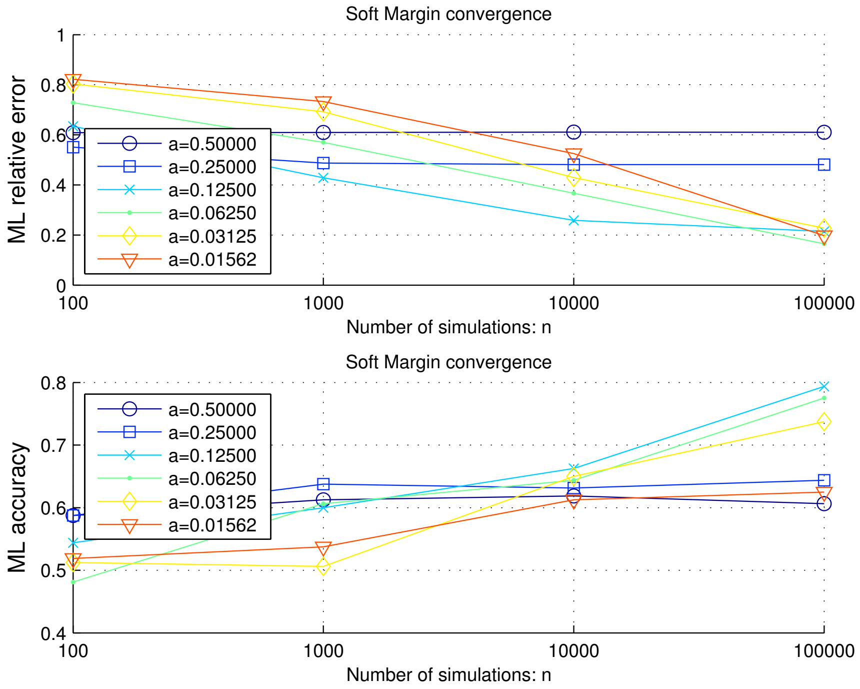


Supplementary Figure 8: Comparison of Soft Margin estimators with different weights $a$ with respect to the Maximum Likelihood relative probability estimation error (plot A) and Maximum Likelihood accuracy (plot B) using the average over 160 different benchmark cases. Benchmark cases were calculated on a small regular network (4-connected grid $N = 30 \times 30$) and SIR process with different parameters $(p, q, T)$ with the direct Monte Carlo estimator with $[10^6 - 10^8]$ simulations per source depending on convergence condition.

## 4 Benchmark dataset

Together with this manuscript, we provide a set of SIR realizations along with their inverse solutions represented as probability over potential candidate nodes. We provide 160 benchmark realizations(downloadable here [2]) on a small regular network (4-connected grid $N = 30 \times 30$) for different SIR parameters:$A = (p = 0.3, q = 0.3, T = 5)$, $B = (p = 0.3, q = 0.7, T = 5)$, $C = (p = 0.7, q = 0.3, T = 5)$ and $D = (p = 0.7, q = 0.7, T = 5)$. The realizations are in the textual form with the following format:

```
-------------------------------
file: realization_2.txt
-------------------------------
#source: 159
#p: 0.700000
#q: 0.700000
#T: 5
#node states:
0
1
0
1
-------------------------------
```

Each realization contains the inverse solution $P(\Theta = \theta_i|\vec{R} = \vec{r}_*)$ calculated with the direct Monte Carlo estimator with $[10^6 - 10^8]$ simulations per source depending on the convergence condition. The convergence condition is relative ML node error: $|P^{2x}_{ML} - P^{x}_{ML}|/P^{2x}_{ML} \leq 0.05$ and the maximal absolute error for all other nodes: $|P^x_i - P^{2x}_i| \leq 0.05$. The solutions are provided in textual form with the following format:

```
------------------------------------------------------------
file: inverse_solution_2.txt
------------------------------------------------------------
#Number of simulation: 10000000
#Node source probabilities:
0.000000
0.240000
0.000000
0.110000
0.000000
------------------------------------------------------------
```

The network is given in the gml network format.

[2] http://lis.irb.hr/epidemic/

# 5 Soft Margin implementation details

In this section, we explain in more details: (i) how to set the Soft Margin width parameter $a$ and (ii) how we relax the assumption on epidemic starting moment $t_0$ by marginalization of conditional probabilities. Let us recall how we calculate source probability distribution via Bayes formula:

$$P(\Theta = \theta_i|\vec{R} = \vec{r_*}) = \frac{P(\vec{R} = \vec{r_*}|\Theta = \theta_i)P(\Theta = \theta_i)}{\sum_{\theta_j} P(\vec{R} = \vec{r_*}|\Theta = \theta_j)P(\Theta = \theta_j)}, \tag{4}$$

and since our prior source probabilities are equal we get:

$$P(\Theta = \theta_i|\vec{R} = \vec{r_*}) = \frac{P(\vec{R} = \vec{r_*}|\Theta = \theta_i)}{\sum_{\theta_j} P(\vec{R} = \vec{r_*}|\Theta = \theta_j)}. \tag{5}$$

Now, the Soft Margin estimates the likelihood via the following formula:

$$\hat{P}(\vec{R} = \vec{r_*}|\Theta = \theta) = \int_0^1 w_a(x)\hat{f}_\theta(x)\mathrm{d}x = \int_0^1 w_a(x) \underbrace{\frac{1}{n}\sum_{i=1}^{n} \delta\left(x - \varphi(\vec{r_*}, \vec{r}_{\theta,i})\right)}_{\hat{f}_\theta(x)} \mathrm{d}x, \tag{6}$$

which can be simplified by using the property of delta distribution: $\int_{-\infty}^{\infty} f(x)\delta(x-b)\mathrm{d}x = f(b)$,

$$\hat{P}(\vec{R} = \vec{r_*}|\Theta = \theta) = \frac{1}{n}\sum_{i=1}^{n}\int_0^1 w_a(x)\delta\left(x - \varphi(\vec{r_*}, \vec{r}_{\theta,i})\right)\mathrm{d}x = \frac{1}{n}\sum_{i=1}^{n} w_a(\varphi(\vec{r_*}, \vec{r}_{\theta,i})). \tag{7}$$

We use the following weighting form: $w_a(x) = e^{-(x-1)^2/a^2}$ and thus the likelihood estimation is equal to:

$$\hat{P}(\vec{R} = \vec{r_*}|\Theta = \theta) = \frac{1}{n}\sum_{i=1}^{n} e^{\frac{-(\varphi(\vec{r_*}, \vec{r}_{\theta,i})-1)^2}{a^2}}. \tag{8}$$

Simplified, for each potential candidate $\theta$, by simulations we obtain $n$ samples of variable $\varphi(\vec{r_*}, \vec{R}_\theta)$: $\{\varphi_{\theta,1}, \varphi_{\theta,2}, ...\varphi_{\theta,n}\}$ from which we calculate the source likelihood: $\hat{P}(\vec{R} = r_*|\Theta = \theta) = \frac{1}{n}\sum_{i=1}^{n} e^{-(\varphi_{\theta,i}-1)^2/a^2}$.

Now, after we calculate $\hat{f}_\theta(x)$ for every potential source, we recalculate the source probability distribution for different values of parameter $a$ in range: $\{1/2, (1/2)^2, (1/2)^3, ..., (1/2)^{15}\}$. Then, we measure the convergence property of estimated PDFs: $\hat{P}_a^n(\Theta = \theta_i|\vec{R} = \vec{r_*})$ for different values of Soft Margin weight $a$ and different number of simulations $n$. Then we choose the parameter $a$ as the minimum of the set of parameters for which the PDFs have converged. We use the following convergence condition for the source PDFs: $|\hat{P}_a^n(\Theta = \theta_{MAP}|\vec{R} = \vec{r_*}) - \hat{P}_a^{2n}(\Theta = \theta_{MAP}|\vec{R} = \vec{r_*})| \leq 0.05$, where $\theta_{MAP}$ is the node $i$ with the maximum estimated source probability in $\hat{P}_a^{2n}(\Theta = \theta_i|\vec{R} = \vec{r_*})$. The smaller the parameter $a$, the estimations becomes more similar to the direct Monte Carlo estimator if the PDFs have converged. Note, that the maximum likelihood (ML) node is the same as the maximum posteriori (MAP) node if our prior source probabilities are equal. As the computational complexity of calculating $\hat{f}_\theta(x)$ is a few orders of magnitude higher than complexity of recalculating source PDF for different parameters $a$, one does not need to set parameter $a$ in advance but rather choose the near-optimal value of $a$ for specific number of simulations $n$.

Up to this point we have assumed that the epidemic duration $T$ or starting point $t_0$ were given in advance. Strictly speaking we should have written the parameter $T$ in all the conditional probabilities $P(\vec{R}=r_*|\Theta=\theta, T=t-t_0)$ instead of just $P(\vec{R}=r_*|\Theta=\theta)$, but this would just complicate the notation since we could also put other given parameters like $G$, $p$ and $q$ in the condition. Instead, unless otherwise stated, we assume that parameters: $T$, $G$, $p$ and $q$ are given. Now we explain how to relax the assumption on specific epidemic parameters. For example, if we know the time $t$ when the realization was observed, but the epidemic starting moment $t_0$ is not known in advance, by marginalization over all possible $t_0$ outcomes we get:

$$P(\vec{R}=\vec{r_*}|\Theta=\theta)=\sum_{t_0=0}^{t} P(\vec{R}=\vec{r_*}, T=t-t_0|\Theta=\theta), \tag{9}$$

where the variable $T$ denotes the epidemic duration. This expression can be further transformed into:

$$P(\vec{R}=\vec{r_*}|\Theta=\theta)=\sum_{t_0=0}^{t} P(\vec{R}=\vec{r_*}|\Theta=\theta, T=t-t_0)P(T=t-t_0|\Theta=\theta). \tag{10}$$

Now, the term $P(\vec{R}=\vec{r_*}|\Theta=\theta, T=t-t_0)$ can be calculated with the Soft Margin estimator like before, and the term $P(T=t-t_0|\Theta=\theta)$ denotes the prior distribution of epidemic duration or epidemic start. But, we do not estimate $\hat{P}(\vec{R}=\vec{r_*}|\Theta=\theta)$ by definition due to its computational cost, but rather by another sample estimation. First, we sample a $T_i$ from the prior probability distribution $P(T=t-t_0|\Theta=\theta)$ and then obtain the sample realization $\vec{r}_{\theta,i}$ for a given $T_i$. We repeat the procedure $n$ times, obtain $n$ temporal samples $\{T_1, ..., T_n\}$ and obtain $n$ corresponding realizations $\{\vec{r}_1, ..., \vec{r}_n\}$. Then, we estimate $\hat{P}(\vec{R}=r_*|\Theta=\theta)$ with the Soft Margin estimator from $n$ realizations: $\{\vec{r}_1, ..., \vec{r}_n\}$ from their similarities to the observed realization: $\{\varphi(\vec{r_*}, \vec{r}_{\theta,1}), ...\varphi(\vec{r_*}, \vec{r}_{\theta,n})\}$.

$$\hat{P}(\vec{R}=r_*|\Theta=\theta)=\sum_{t_0=0}^{t} \hat{P}(\vec{R}=r_*|\Theta=\theta, T=t-t_0)\underbrace{\hat{P}(T=t-t_0|\Theta=\theta)}_{\frac{k_i}{n}}$$

If we regroup $k_i$ realizations with the same $T_i$ we get:

$$\hat{P}(\vec{R}=r_*|\Theta=\theta)=\sum_{t_0=0}^{t} \underbrace{\sum_i \frac{1}{k_i} e^{\frac{-(\varphi(\vec{r_*}, \vec{r}_{\theta,i})-1)^2}{a^2}}}_{Soft\ Margin} \frac{k_i}{n}=\frac{1}{n}\sum_{i=1}^{n} e^{\frac{-(\varphi(\vec{r_*}, \vec{r}_{\theta,i})-1)^2}{a^2}}.$$

Together with this manuscript, we provide the C++ implementation code of the Soft Margin and other estimators (downloadable here [3]).

[3] http://lis.irb.hr/epidemic/

## 6 Pruning and Soft Margin

The Soft Margin estimator uses the following realization similarity weighting function: $w_a(x) = e^{-(x-1)^2/a^2}$. Now, if we have the following weighting function $w_a^{'}(x)$, that has a cut-off at point $x = \varphi_B$ defined with the following formula:

$$w_a^{'}(x) = \begin{cases} w_a(x) = e^{-(x-1)^2/a^2} & : x \geq \varphi_B, \\ 0 & : x < \varphi_B. \end{cases}, \tag{11}$$

then we can introduce the pruning mechanism for terminating the simulation at time $t$ before the stopping point $T$ with no effect on the likelihood estimation with the weighting function $w_a^{'}(x)$.

Let us recall the definition of the error term for every simulated realization $\vec{r_i^t}$ at some point in time $t < T$ w.r.t observed realization $\vec{r_*^T}$ at time $T$:

$$\epsilon_t^B(\vec{r_i^t}, \vec{r_*^T}) = \frac{1}{N} \sum_{k \in V} \psi_\wedge(1 - \vec{r_*}^T(k), \vec{r_i}^t(k)), \tag{12}$$

where $\psi_\wedge(x_1, x_2)$ function is defined as the binary "AND" function:

$$\psi_\wedge(x_1, x_2) = \begin{cases} 1 & : (x_1 = 1 \text{ and } x_2 = 1), \\ 0 & : \text{else}. \end{cases} \tag{13}$$

**Lemma** The error term $\epsilon_t^B(\vec{r_i^t}, \vec{r_*^T})$ is monotonic increasing function w.r.t. time $t+1, t+2, ..., T$.

**Proof** Once the node goes from susceptible state $\vec{r_i^t}(k) = 0$ at time $t$, it cannot come back for any time after $t$ in the SIR model or any other compartmental model with no recurrent states.

**Proposition** The contribution of all realizations $\vec{r_i^t}$ at time $t < T$ to the likelihood estimation at time $T$ is zero if the $\epsilon_t^B(\vec{r_i^t}, \vec{r_*^T}) > (1-\varphi_B)$, where the term $(1-\varphi_B)$ denotes the maximal error term we can have.

**Proof** We need to prove that $\epsilon_t^B(\vec{r_i^t}, \vec{r_*^T}) > (1-\varphi_B)$ implies $\varphi_i^T < \varphi_B$, where $\varphi_i^T$ denotes the similarity of realization $\vec{r_i^T}$ at time $T$. The connection between error terms and (XNOR) similarity is the following:

$$N(1 - \varphi_i^t) = N - \sum_{k \in V} \psi_\oplus(\vec{r_*}^T(k), \vec{r_i}^t(k))$$

Recall the definition of the XNOR $\psi_\oplus(x_1, x_2)$ function:

$$\psi_\oplus(x_1, x_2) = \begin{cases} 1 & : (x_1 = 1 \text{ and } x_2 = 1) \text{ or } (x_1 = 0 \text{ and } x_2 = 0), \\ 0 & : \text{else}. \end{cases} \tag{14}$$

$$N(1 - \varphi_i^t) = \sum_{k \in V} \psi_\wedge(\vec{r_*}^T(k), 1 - \vec{r_i}^t(k)) + \sum_{k \in V} \psi_\wedge(1 - \vec{r_*}^T(k), \vec{r_i}^t(k))$$

$$\implies (1 - \varphi_i^t) = \underbrace{\frac{1}{N} \sum_{k \in V} \psi_\wedge(\vec{r_*}^T(k), 1 - \vec{r_i}^t(k))}_{\epsilon_t^A} + \underbrace{\frac{1}{N} \sum_{k \in V} \psi_\wedge(1 - \vec{r_*}^T(k), \vec{r_i}^t(k))}_{\epsilon_t^B}$$

$$(1 - \varphi_i^t) = \epsilon_t^A(\vec{r_i^t}, \vec{r_*^T}) + \epsilon_t^B(\vec{r_i^t}, \vec{r_*^T})$$

Therefore, the total error $1 - \varphi_i^t$ has two components: $\epsilon_t^A$ and $\epsilon_t^B$. Now, if we assume that $\epsilon_t^B(\vec{r_i^t}, \vec{r_*^T}) > (1 - \varphi_B)$ from previous lemma, we conclude that $\epsilon_T^B(\vec{r_i^t}, \vec{r_*^T}) > (1 - \varphi_B)$ and if we add non-negative error term to the left side of previous inequality we get:

$$\epsilon_T^A(\vec{r_i^t}, \vec{r_*^T}) + \epsilon_T^B(\vec{r_i^t}, \vec{r_*^T}) > (1 - \varphi_B) \implies (1 - \varphi_i^T) > (1 - \varphi_B) \implies \varphi_i^T < \varphi_B.$$

Therefore, if at time $t$ the error term $\epsilon_t^B(\vec{r_i^t}, \vec{r_*^T}) > (1 - \varphi_B)$ then at time $T$ the similarity $\varphi_i^T$ can only be lower than the border cutoff value $\varphi_B$.

**Corollary** Monte Carlo SIR realization simulation $\vec{r_i^t}$ at time $t < T$ can be terminated if the $\epsilon_t^B(\vec{r_i^t}, \vec{r_*^T}) > (1 - \varphi_B)$ as it will have no contribution to the likelihood calculated by weighted function $w_a^{'}(x)$ with a cutoff at $\varphi_B$.

# 7 Soft Margin time complexity

The average run-time complexity $\overline{RT}$ of Soft Margin estimator is:

$$\overline{RT} \propto |\vec{r_*}| \times n \times \overline{RT}_M,$$

where the term $|\vec{r_*}|$ denotes the number of potential sources in the observed realization, the term $n$ denotes number of samples of the random variable $\vec{R}_\theta$ or alternatively the number of simulations of a contagion process and $\overline{RT}_M$ denotes the average run-time complexity of sampling one realization from contagion process $M$. Sampling the realizations from a contagion process in our case is equal to one Monte Carlo simulation of stochastic contagion model and returning one realization vector $\vec{r}_{\theta,i}$. Note that in the worst-case scenario the number of potential sources is proportional to the network size $|\vec{r_*}| \propto N$, but in reality we are mostly interested in source detection problem when the number of potential sources is much smaller than the network size.
Note, that the calculations of likelihood for different sources $\theta$ in $\vec{r_*}$ are computed in scalable parallel way with the MapReduce paradigm. The "Map" step distributes the source independent problems to worker nodes and "Reduce" step collects likelihood estimators and provides source probability distribution.
In the case when contagion process is the SIR model on an arbitrary static network, the average run-time complexity for single SIR discrete simulation (NaiveSIR algorithm [2]) is:

$$\overline{RT}_{M1} \propto E(X_T) \times \overline{k} \times T,$$

where the term $E(X_T)$ denotes the expected number of infected nodes up to temporal threshold $T$ and $\overline{k}$ is the average node degree.
In the case when the contagion process is the SIR model on temporal network, the run-time complexity for single SIR discrete simulation is:

$$\overline{RT}_{M2} \propto L_T,$$

where $L_T$ denotes the number of interactions during epidemic process with duration $T$.
Note that after we have calculated the estimated PDF for each potential candidate node $\hat{f}_\theta(x)$, we can estimate source probabilities for different weight parameters $a$ since this step is far less demanding than the previous steps.

Supplementary Table 1: **The source detection execution times on an empirical temporal network [3]. Execution times of source detection are measured with parallel computation on 50 CPU cores on the AMD Opteron(tm) Processor 6380, 2.5 GHz each. The computations are done in parallel by using a high performance Message Passing Library with the C++ language. Averaging was done over 50 independent experiments where the initial moment $t_0$ was chosen in period between $[100-200]$ days, the initial source was randomly selected from the set of active nodes in $t_0$ moment with the SIR STD model ($p = 0.3, q = 0.01$) and realization $\vec{r_*}$ was observed at time $t = 300$ days. The run times are averaged over 50 independent experiments with the mean realization size $|\vec{r_*}|$ equal to 86. We have used the Soft Margin estimator, where the width parameter $a$ was chosen as a minimum of parameters from set: $\{1/2, (1/2)^2, (1/2)^3, ..., (1/2)^{15}\}$ for which the ML estimate converged up to 0.05 of relative change between consecutive simulations.**

| Number of simulations | n = 5000 | n = 10000 | n = 15000 | n = 20000 |
|---|---|---|---|---|
| Mean time [s] | 2.9 | 5.8 | 8.7 | 11.6 |

# 8 Empirical temporal network – description

The dataset (for more details see [3],[4]) used in the main paper is the approximation of empirical temporal sexual network gathered from the public online forum in Brazil. The dataset consists out of the triplets $(v_i, v_j, t)$, which represents the event that the nodes $v_i$ (male) and $v_j$ (female prostitute) had a sexual interaction at a time $t$ based upon the evaluation and comments from the posts on the forum. The forum is represented by the bipartite network which connects (sex buyers) posting a forum thread to the escort (sex sellers) discussed in the thread. The dataset spans from the period of September 2002 until October 2008 with the 50 185 contacts between 6642 escorts and 10106 males in twelve Brazilian cities. Like the authors in original case study [3], we also discard the initial 1000 days in the data to a transient period with sparse contacts.

**Disclaimer**: We have used the published existing dataset of sexual contacts in high-end prostitution because it contains valuable and rarely available information on temporal network of contacts serving as pathways of STD spreading. It is important to note that the use of this dataset does not reflect the authors' views, opinions and attitudes on prostitution and it does not in any way imply that the authors support the activities documented in the dataset or the way the data were gathered.

# 9 Source detection on temporal networks

In this section, we show the results for source detection on the empirical temporal networks for contagion with the SIR model with high transmission probability $p = 0.8$ with recovery parameter $q = 0.05$ (expected recovery is 20 days). In Supplementary Figure 9 plot A, we show the results when starting $t_0$ was uniformly chosen from the interval $[100-200]$ day, the end of epidemic was set to the day $t = 300$ and we used different uniform priors ($\epsilon$) on $t_0$ moment. Plot B in the Supplementary Figure 9 demonstrates the effect of detecting the source node from network with randomized temporal ordering with parameter $\Delta$.

In all the cases so far, we have assumed that we know the states of all the nodes in the network at the temporal snapshot $t$. Now, we will show that we can relax that assumption. We will assume that we can only observe the states of a random subset $O \subseteq V$ of all the nodes in the network. In Supplementary Figure 10, we show the performance results for the source detection of STD disease when we know the states of 100%, 50% and 20 % of all the nodes in the network chosen randomly. Realization vectors $\vec{r_*}$

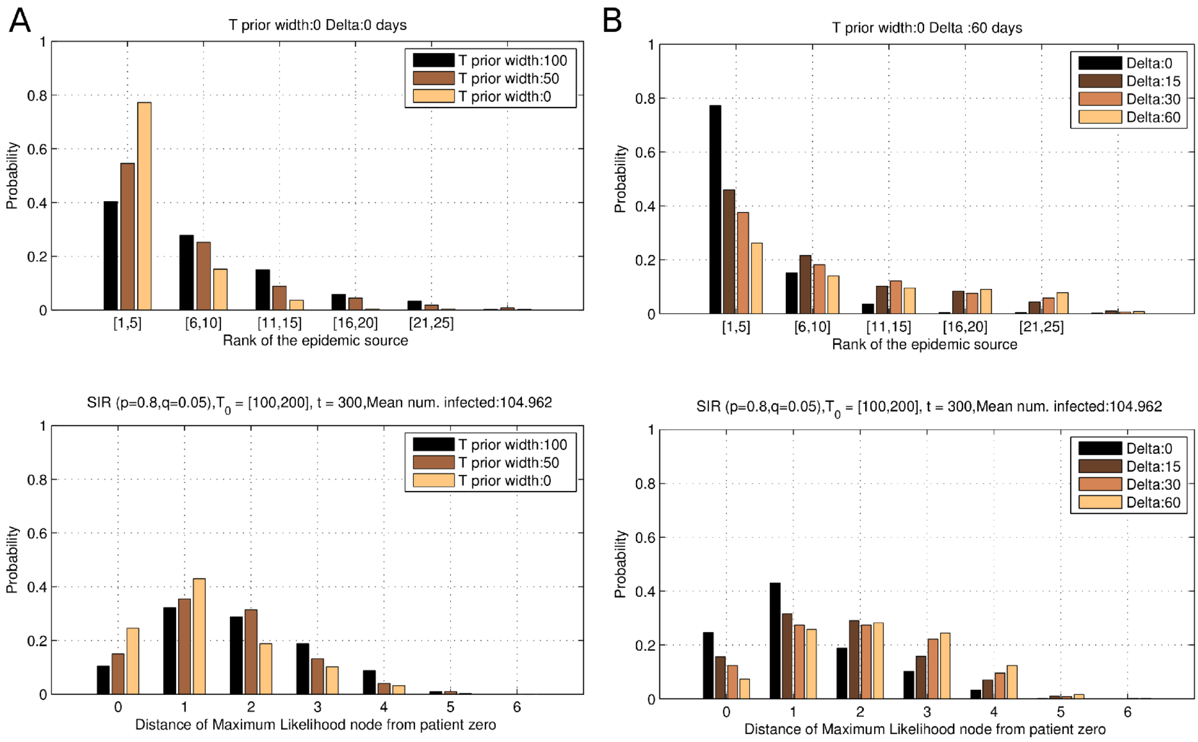


Supplementary Figure 9: The Source detection of simulated sexually transmitted infections spreading in an empirical spatio-temporal network of sexual contacts in Brazil. The experiment consists of 500 experiments where the initial moment $t_0$ was uniformly chosen in period between $[100 - 200]$ days, the initial source was randomly selected from the set of active nodes in the moment $t_0$ with the SIR model $(p = 0.8, q = 0.05)$ and realization $\vec{r_*}$ was observed at time $t = 300$ day. Plot A: The influence of prior knowledge about initial outbreak moment $[t_0 - \epsilon, t_0 + \epsilon]$ . Plot B: The influence of detecting the source node from temporal networks with randomized temporal ordering of interactions within $\Delta$ days.

now can have the following values: $\{0, 1, ?\}$, where the "?" denotes the unknown state. In order to apply our methodology, we only need to adopt the similarity function in a way that it can handle the unknown states and determine the set of potential candidate sources $S$. We use the same similarity function like in the main manuscript (Jaccard similarity), but we neglect the comparison with the missing state "?". The set of potential candidates is the union of all the nodes with state "1" and all the nodes with state "?" which are not surrounded with neighbours with "0" state only (they cannot be the initial source).

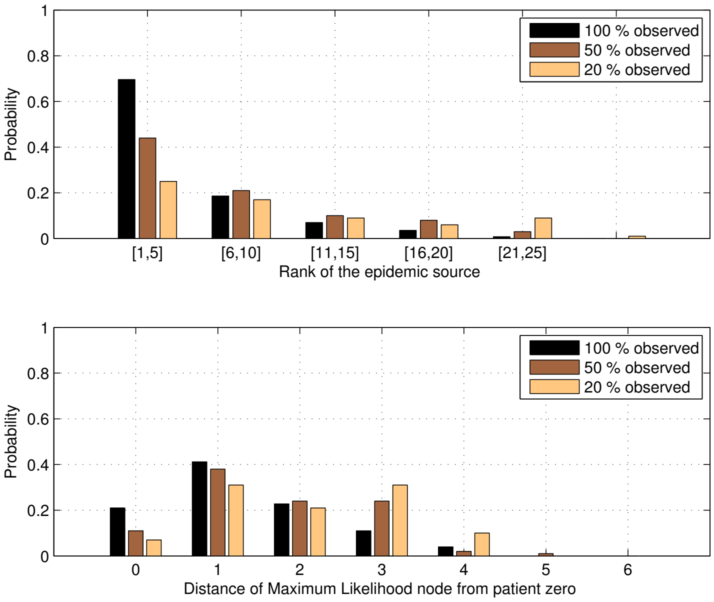


Supplementary Figure 10: The Source detection of simulated sexually transmitted infections spreading in an empirical spatio-temporal network of sexual contacts in Brazil when we know the states of 100%, 50% and 20 % of all the nodes in the network chosen randomly. The experiment consists of 100 experiments where the initial moment $t_0$ was uniformly chosen in period between $[100-200]$ days, the initial source was randomly selected from the set of active nodes in the moment $t_0$ with the SIR model $(p = 0.3, q = 0.01)$ and realization $\vec{r_*}$ was observed at time $t = 300$ day.

## 10 Detectability regimes

In this section, we show the existence of different detectability regimes under different conditions on the regular 4-connected lattice. First, we show that the SIR process has different detectability regimes (see Figure 11) low detectability-high entropy region $(p < 0.2)$, intermediate detectability-intermediate entropy region $(0.2 < p < 0.7)$ and high detectability-low entropy region $(p > 0.7)$.

Then, we show the effect of network size (see Figure 12) for a fixed stopping time $T$. In a regime, when the network size restricts the epidemic spreading but not the epidemic itself via it's natural evolution characterized by the parameters $(p, q)$ or stopping time $T$, the entropy is high as the realizations from different sources are almost identical. Our experiments confirm that the detection of source is not possible in this regime (see grid 3x3 in Figure 12). Contrary, when the stopping time $T$ restricts the epidemic spreading, depending on the process parameters $(p, q)$ different sources are likely to produce

disjoint realization ensembles which causes low entropy.

Next, we demonstrate the generality of our findings for different spreading models (see Figure 13) with discrete time up to a fixed stopping time $T$:

- SI model: Susceptible-Infected model. At each time step an infected node can infect a neighbouring susceptible node with probability $p$.
- SIR model: Susceptible-Infected-Recovered model- At each time step an infected node can infect a neighbouring susceptible node with probability $p$ and a infected node recovers with probability $q$.
- IC model: Independent-Cascade model was proposed by Kempe, Kleinberg and Tardos in 2003. An infected node infects its susceptible neighbour with probability $p$ independently of all other nodes. Moreover, each infected node has just one chance to infect its neighbours.
- ISS model: Ignorant-Spreading-Stifler model. This information/rumor spreading model divides the individuals into three groups: ignorants, who have not heard the information/rumor, spreaders, who are propagating the information/rumor to ignorants and stiflers, who know the information/rumor and are no longer propagating it. The probability of spreading the information/rumor from spreaders to ignorants is $a$ in one discrete time step. If the spreader interacts with spreader or stifler it turns to stifler state with probability $b$.

Note, that we did not choose the parameter $a$ for kernel estimation width of the Soft Margin estimator in advance. The parameter $a$ was taken as a result of optimization, the minimum $a$ from for which the source PDFs have converged. After we calculate $\hat{f}_\theta(x)$ for every potential source, we evaluate the source probability likelihood estimations for different values of parameter $a$ in range: $\{1/2, (1/2)^2, (1/2)^3, ..., (1/2)^{15}\}$. Then, we measure the convergence property of estimated PDFs: $\hat{P}^n_a(\Theta = \theta_i|\vec{R} = \vec{r}_*)$ for different values of Soft Margin weight $a$ and different number of simulations $n$ ($10^4$ - $10^6$). Then we choose the parameter $a$ as the minimum of the set of parameters for which the PDFs have converged. We use the following convergence condition for the source PDFs: $|\hat{P}^n_a(\Theta = \theta_{MAP}|\vec{R} = \vec{r}_*) - \hat{P}^{2n}_a(\Theta = \theta_{MAP}|\vec{R} = \vec{r}_*)| \leq 0.1$, where $\theta_{MAP}$ is the node $i$ with the maximum estimated source probability in $\hat{P}^{2n}_a(\Theta = \theta_i|\vec{R} = \vec{r}_*)$. The smaller the parameter $a$, the estimations becomes more similar to the direct Monte Carlo estimator if the PDFs have converged.

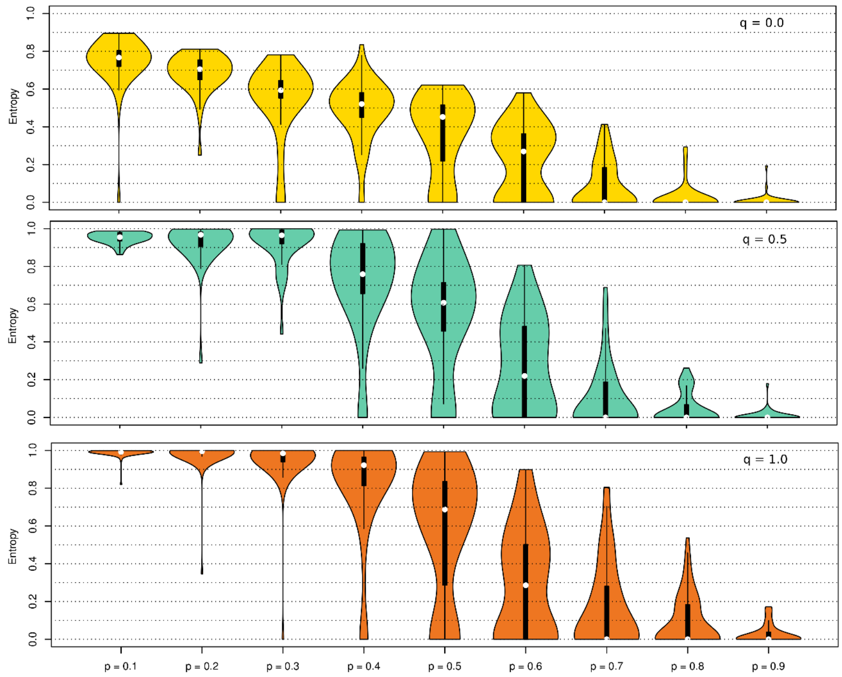


Supplementary Figure 11: Box plots with estimated entropy density functions of entropy of source probability distributions for potential candidates on the 4-connected lattice ($N = 30 \times 30$ nodes) calculated with the Soft Margin method with $10^4 - 10^6$ simulations per source for different parameters: $p$ in range $0.1 - 0.9$, three values of $q$: $(0.0, 0.5, 1.0)$ and fixed stopping time point $T = 5$. Soft Margin estimator with adaptive width $a$ (minimal $a$ for which source PDFs have converged) with the number of simulations in range: $10^4 - 10^6$ (few orders less than with Direct Monte Carlo).

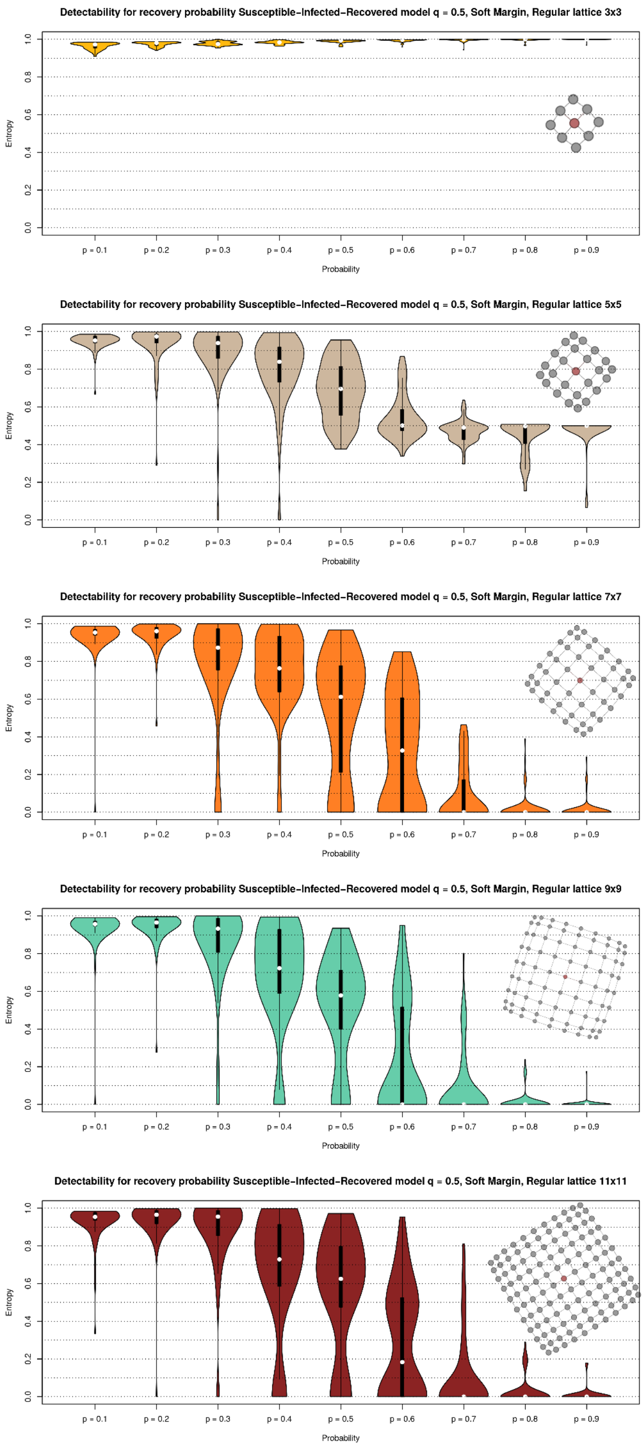


Supplementary Figure 12: Box plots with estimated entropy density functions of entropy of source probability distributions for potential candidates on the 4-connected lattice of different sizes calculated with the Soft Margin method with $10^4 - 10^6$ simulations with adaptive $a$ per source for different parameters: $p$ in range $0.1 - 0.9$, $q = 0.5$ and fixed stopping point $T = 5$. The node denoted with red colour is the source node in each experiment.

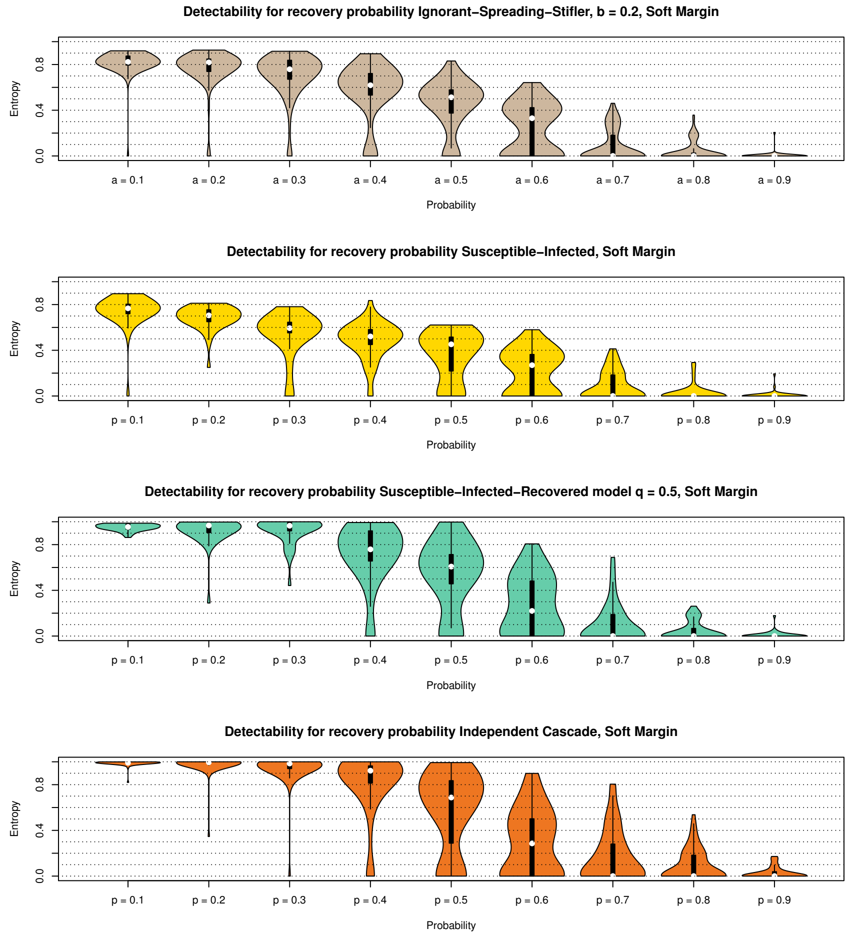


Supplementary Figure 13: Box plots with estimated entropy density functions of entropy of source probability distributions for potential candidates on the 4-connected lattice ($N = 30 \times 30$ nodes) calculated with the Soft Margin method with $10^4 - 10^6$ simulations per source for different spreading models: ISS, SI, SIR and IC and different parameters for a fixed stopping point $T = 5$. Soft Margin estimator with adaptive width $a$ (minimal $a$ for which source PDFs have converged).

## References


[1] Lokhov AY, Mezard M, Ohta H, Zdeborova L (2014) Inferring the origin of an epidemy with dynamic message-passing algorithm. Phys. Rev. E 90, 012801

[2] Antulov-Fantulin N, Lancic A, Stefancic H, Sikic M (2013) Fastsir algorithm: A fast algorithm for the simulation of the epidemic spread in large networks by using the susceptible–infected–recovered compartment model. Information Sciences 239: 226 - 240.

[3] Rocha LEC, Liljeros F, Holme P (2011) Simulated epidemics in an empirical spatiotemporal network of 50,185 sexual contacts. PloS Computational Biology 7: e1001109–.

[4] Rocha LEC, Liljeros F, Holme P (2010) Information dynamics shape the sexual networks of internet-mediated prostitution. Proc Natl Acad Sci USA 107: 5706–5711.

[5] Antulov-Fantulin N, Lancic A, Stefancic H, Sikic M, Smuc T (2013) Statistical inference framework for source detection of contagion processes on arbitrary network structures. Proceedings of 2014 IEEE Eighth International Conference on Self-Adaptive and Self-Organizing Systems Workshops.

[6] Zhu, K., Ying, L., (2014) Information Source Detection in the SIR Model: A Sample-Path-Based Approach, IEEE/ACM Transactions on Networking, vol.PP, no.99, pp.1,1

[7] Comin CH, da Fontoura Costa L (2011) Identifying the starting point of a spreading process in complex networks. Phys Rev E 84: 056105.
